# Supplementary material for: Single Pair Cross-Modality Super Resolution
Source: arXiv:2004.09965 source file (2021-01-22)
Supplement: Supplementary file 1 [file appendix.tex]

\input{tex_supp/additional_results}
\input{tex_supp/alternating}

\begin{figure}
%\begin{minipage}[t]{.48\textwidth}
%\centering
\includegraphics[height=70pt,width=\linewidth]{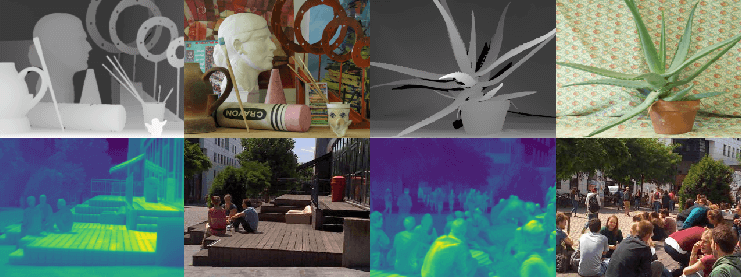}
\caption{The visual-depth pairs from the Middlebury dataset (top row) and the visual-thermal pairs from the ULB17-VT dataset (bottom row) show strong multi-modal registration. Under less than optimal imaging conditions, such alignment is hard to achieve.}
\label{fig:aligned_datasets}
%\end{minipage}
\end{figure}
%\hfill
%\begin{minipage}[t]{.48\textwidth}
\begin{figure}
%\centering
\includegraphics[height=70pt,width=\linewidth]{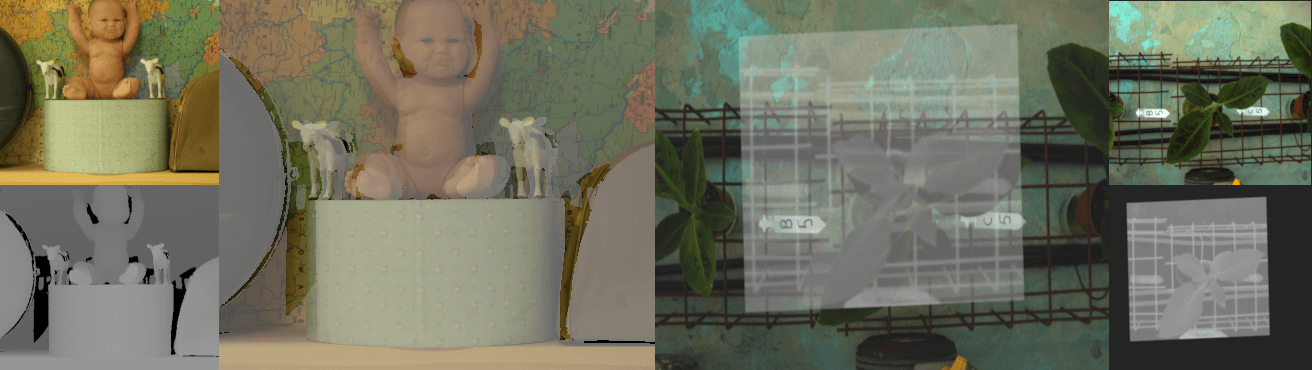}
\caption{Two examples of Weakly Aligned modality pairs. To visualize the misalignment, we overlaid them with semi-transparency. Note, the ghosting effect where cross-modal misalignment occurs.}
\label{fig:misaligned_datasets}
%\end{minipage}
\end{figure}
%\begin{wrapfigure}{r}{0.60\textwidth}
%\centering
%\includegraphics[height=90pt]{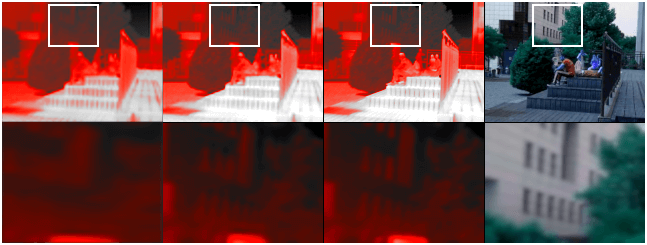}
%\caption{
%From left to right, respectively: Bi-cubic, CMSR (our method), Ground-Truth IR, and the RGB input. Here, CMSR succeeded to produce the building's windows during the SR process, despite never seeing their Thermal (IR) representation.}
%\label{fig:learning_windows}
%\end{wrapfigure}

%\begin{figure}
%\begin{minipage}[t]{.38\textwidth}
%\centering
%\includegraphics[width=165pt]{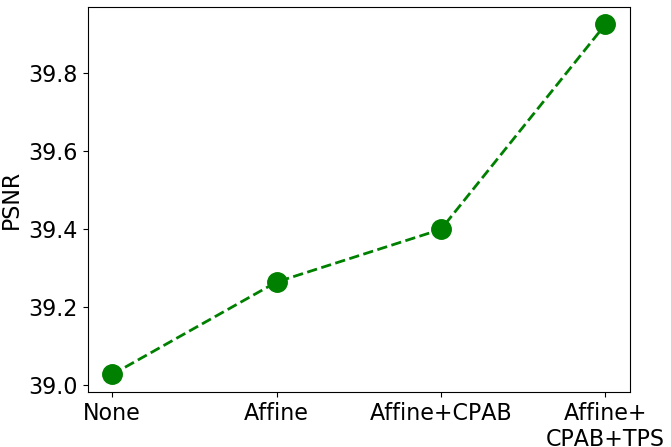}
%\caption{We let CMSR perform $4x$ SR on a Weakly Aligned visual-thermal pair, with different transformation layers, averaged across 5 runs. The results indicate that each layer contributes to the final PSNR, which can also be seen visually in Figure \ref{fig:ablation_deformation_visualisation}}. 
%\label{fig:ablation_deformation_graph}
%\end{minipage}
%\hfill
%\begin{minipage}[t]{.58\textwidth}
%\centering
%\includegraphics[height=80pt,width=\linewidth]{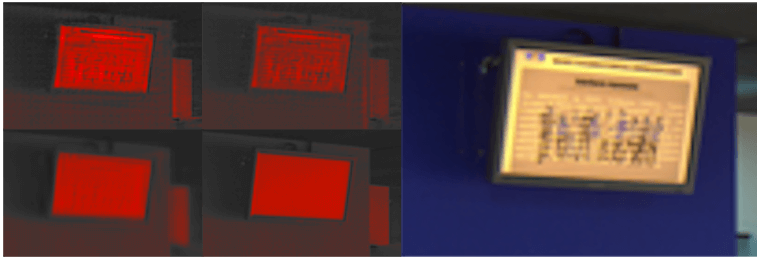}
%\caption{
%CMSR uses its RGB input conservatively. 
%Compared to VTSRCNN (top left) and VTSRGAN (top right), CMSR avoids introducing noticeable redundant artifacts and textures induced by RGB modality. Ground-Truth (bottom right) is given as reference.}
%\label{fig:artifact_comparison}
%\end{minipage}
%\end{figure}

%\centering

%\end{figure}
%\end{minipage}
%\end{wrapfigure}
