# Supplementary material for: Single Pair Cross-Modality Super Resolution
Source: arXiv:2004.09965 source file (2021-01-22)
Supplement: Supplementary file 2 [file deformation.tex]

To show the necessity of each layer of our coarse-to-fine deformation framework (Section 3.1 of the original paper), we evaluated CMSR on a Weakly Aligned pair, adding one layer at a time, averaged across multiple runs. The results indicate that each layer is necessary and plays a different role, which can be seen visually in Figure \ref{fig:ablation_deformation_visualisation}, and numerically in Figure \ref{fig:ablation_deformation_graph}.

Two additional points should be mentioned; First, we remind that our goal is not to perform image registration. Hence, we measure the quality of alignment through the quality of the yielded SR result, and not by conventional image registration metrics. Second, when CMSR is evaluated with no transformation layers on a severely misaligned pair (like the one in Figure \ref{fig:ablation_deformation_visualisation}), its RGB input remains mostly unused, enabling CMSR to produce a result that is comparably worse (as shown in \ref{fig:ablation_deformation_graph}), but does not reflect the failed fusion of misaglined RGB objects. This conservative approach allows our method to surpass competing cross-modal SR methods. CMSR leverages its RGB modality input only when it contributes to the final SR result; when CMSR has no transformation layers, a severely misaligned RGB input will mostly be ignored.

\begin{figure}
\centering
\includegraphics[height=165pt]{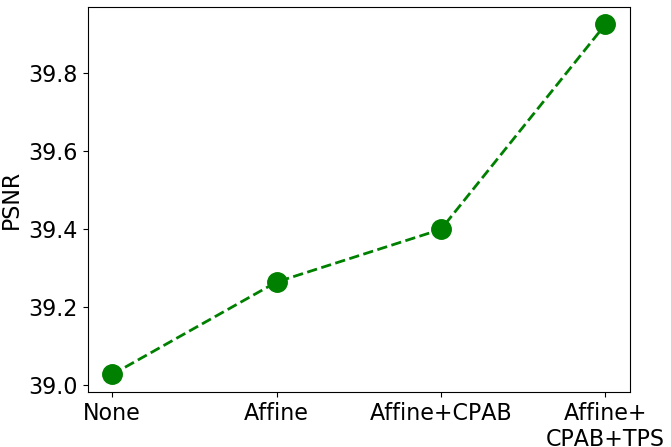}
\caption{We let CMSR perform $4x$ SR on a Weakly Aligned visual-thermal pair, with different transformation layers, averaged across 5 runs. The results indicate that each layer contributes to the final PSNR, which can also be seen visually in Figure \ref{fig:ablation_deformation_visualisation}.}
\label{fig:ablation_deformation_graph}
\end{figure}

\begin{figure*}
\centering
\includegraphics[height=360pt]{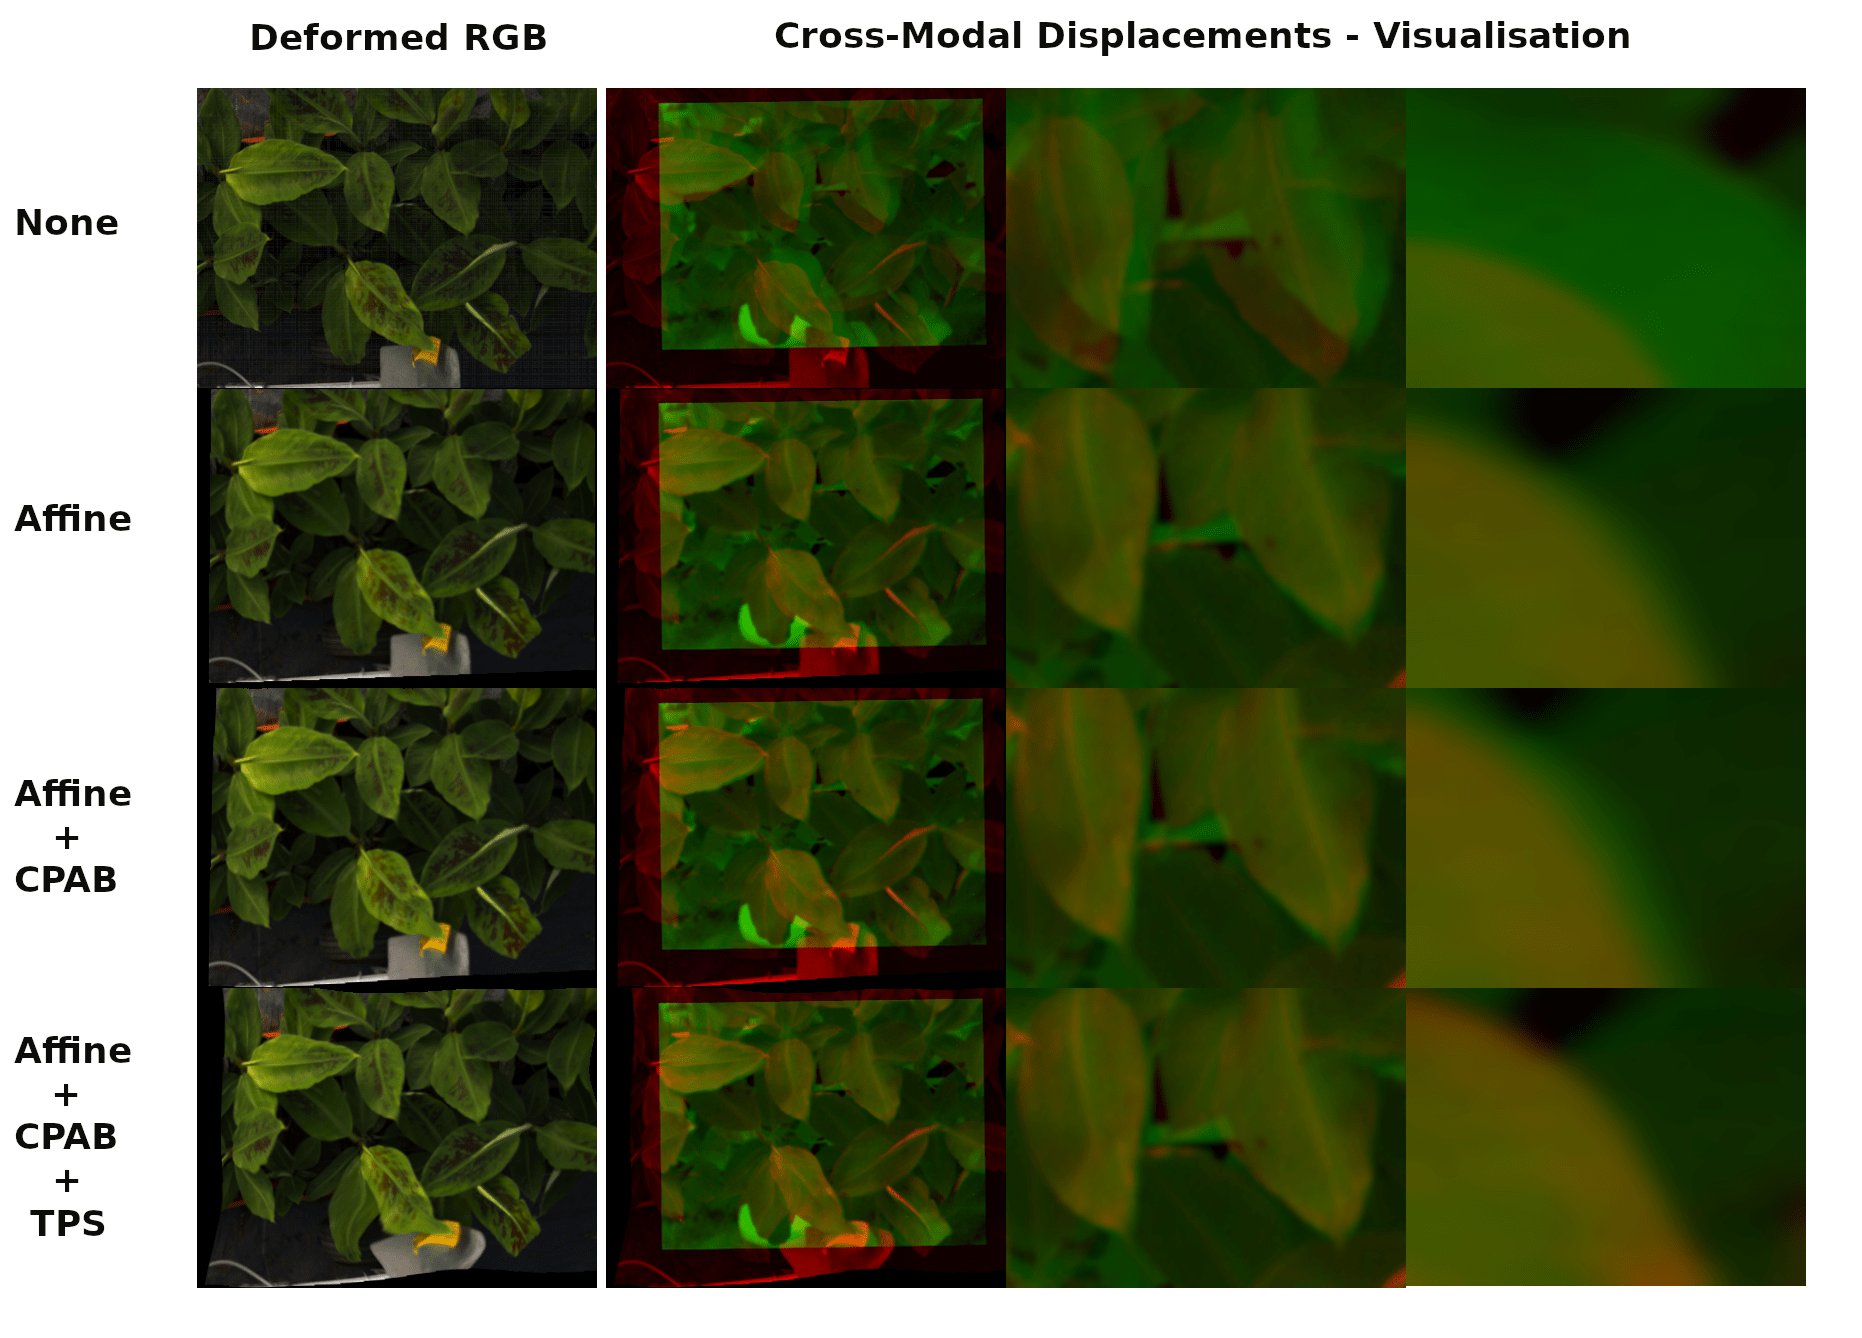}
\caption{We evaluated CMSR using different transformation layers. In the leftmost column, the resulting deformed RGB image is given. In the other columns we show the resulting alignment, visualized through blending of the R-G (Red-Green) channels of the aforementioned deformed RGB image, together with the Ground-Truth thermal image (which is unavailable to CMSR).}
\label{fig:ablation_deformation_visualisation}
\end{figure*}
